# Supplementary material for: The SAMI Galaxy Survey: flipping of the spin-filament alignment correlates most strongly with growth of the bulge
Source: arXiv:2208.10767 ancillary file (2022-08-23)
Supplement: Supplementary file 1 [file SupplementaryFigures.pdf]

# Supplementary Material

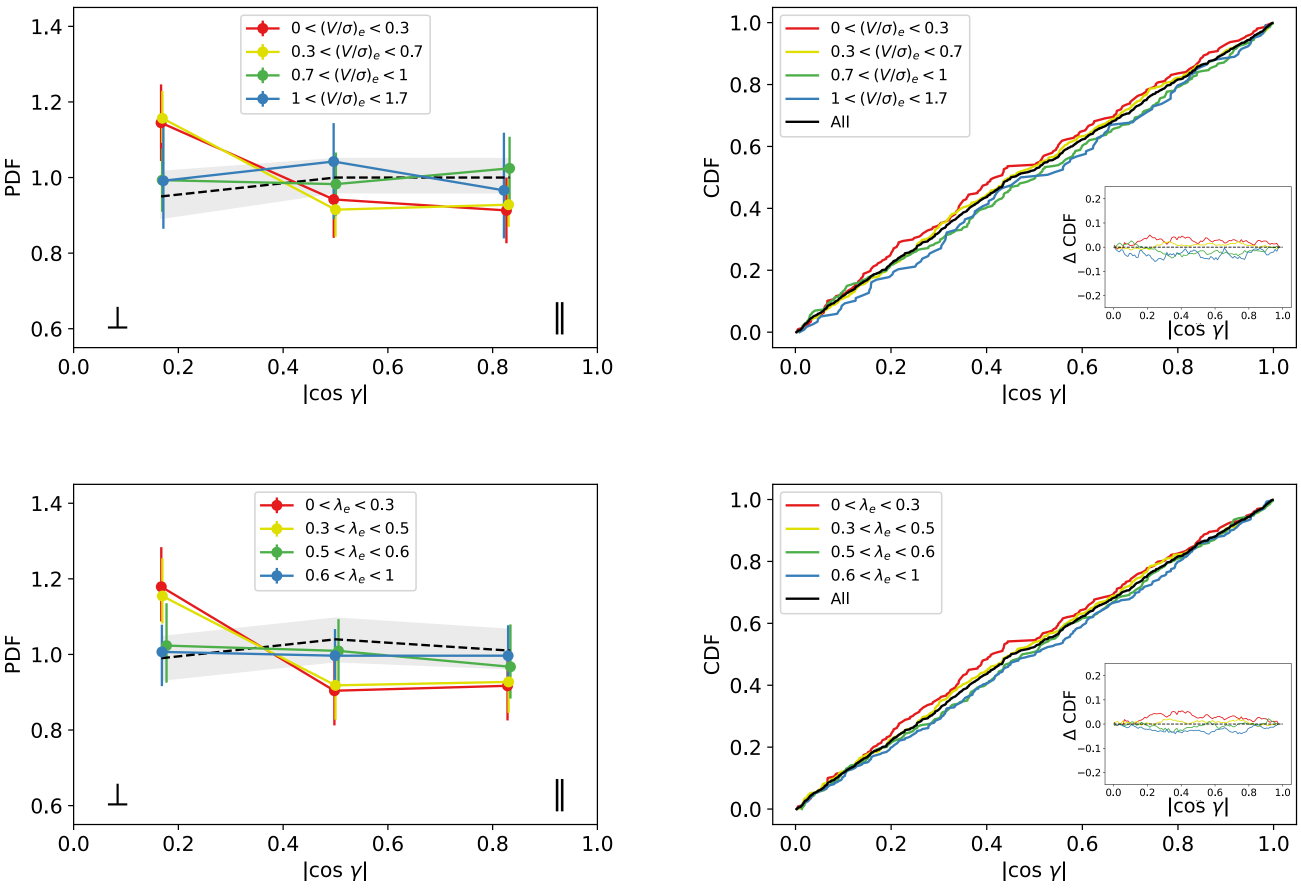


**Figure S1:** PDFs (left) and CDFs (right) of the spin–filament alignments for 1071 SAMI galaxies in ranges of $(V/\sigma)_e$ (top) and $\lambda_e$ (bottom). A statistically significant preference for perpendicular alignments is found for lower $(V/\sigma)_e$ and $\lambda_e$ values. Overall, similar PDFs are found as a function of $(V/\sigma)_e$ and $\lambda_e$.

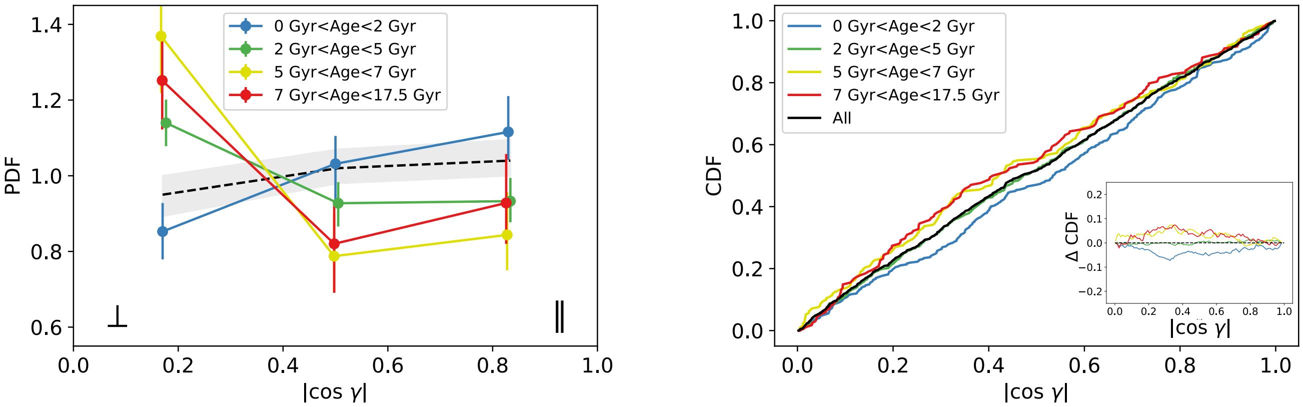


**Figure S2:** PDFs (left) and CDFs (right) of the spin–filament alignments for 1121 SAMI galaxies in ranges of age. A statistically significant preference for perpendicular alignments is found for older galaxies. A significant difference is found between the $|\cos\gamma|$ distributions of the youngest and oldest galaxies.

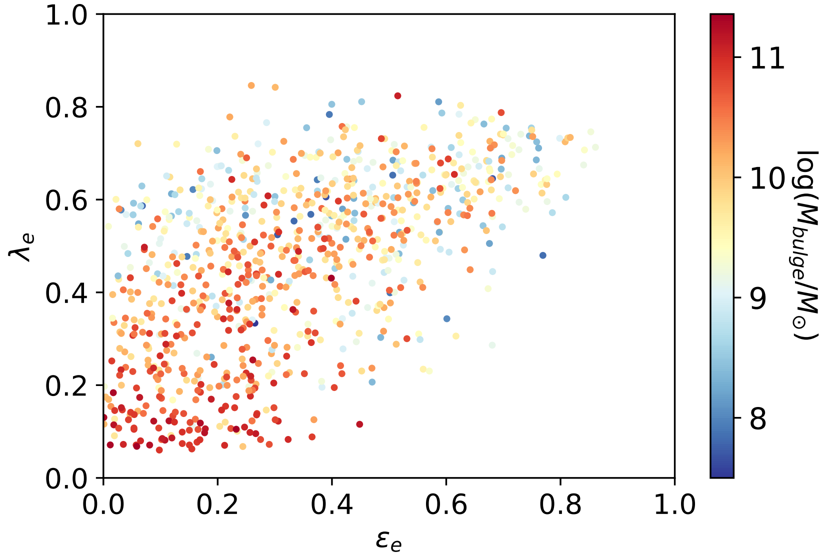


**Figure S3:** The distribution of $\lambda_e$ and ellipticity for 1071 SAMI galaxies, colour-coded according to $M_{\rm bulge}$. Galaxies with $\lambda_e$ <0.5 mostly have high $M_{\rm bulge}$ values, consistent with their significant tendency to perpendicular spin–filament alignments, while galaxies with $\lambda_e$ >0.5 show a broader range in $M_{\rm bulge}$, consistent with their uniform distribution in $|\cos\gamma|$.

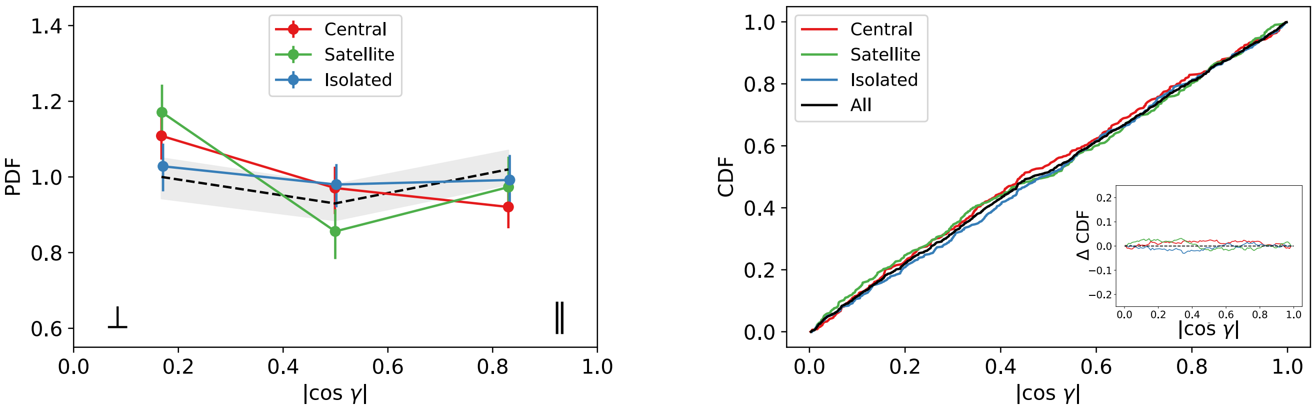


**Figure S4:** PDFs (left) and CDFs (right) of the spin–filament alignments for 1121 SAMI galaxies divided into group centrals, satellites and isolated galaxies. A statistically significant preference for perpendicular alignments is found for group central galaxies.

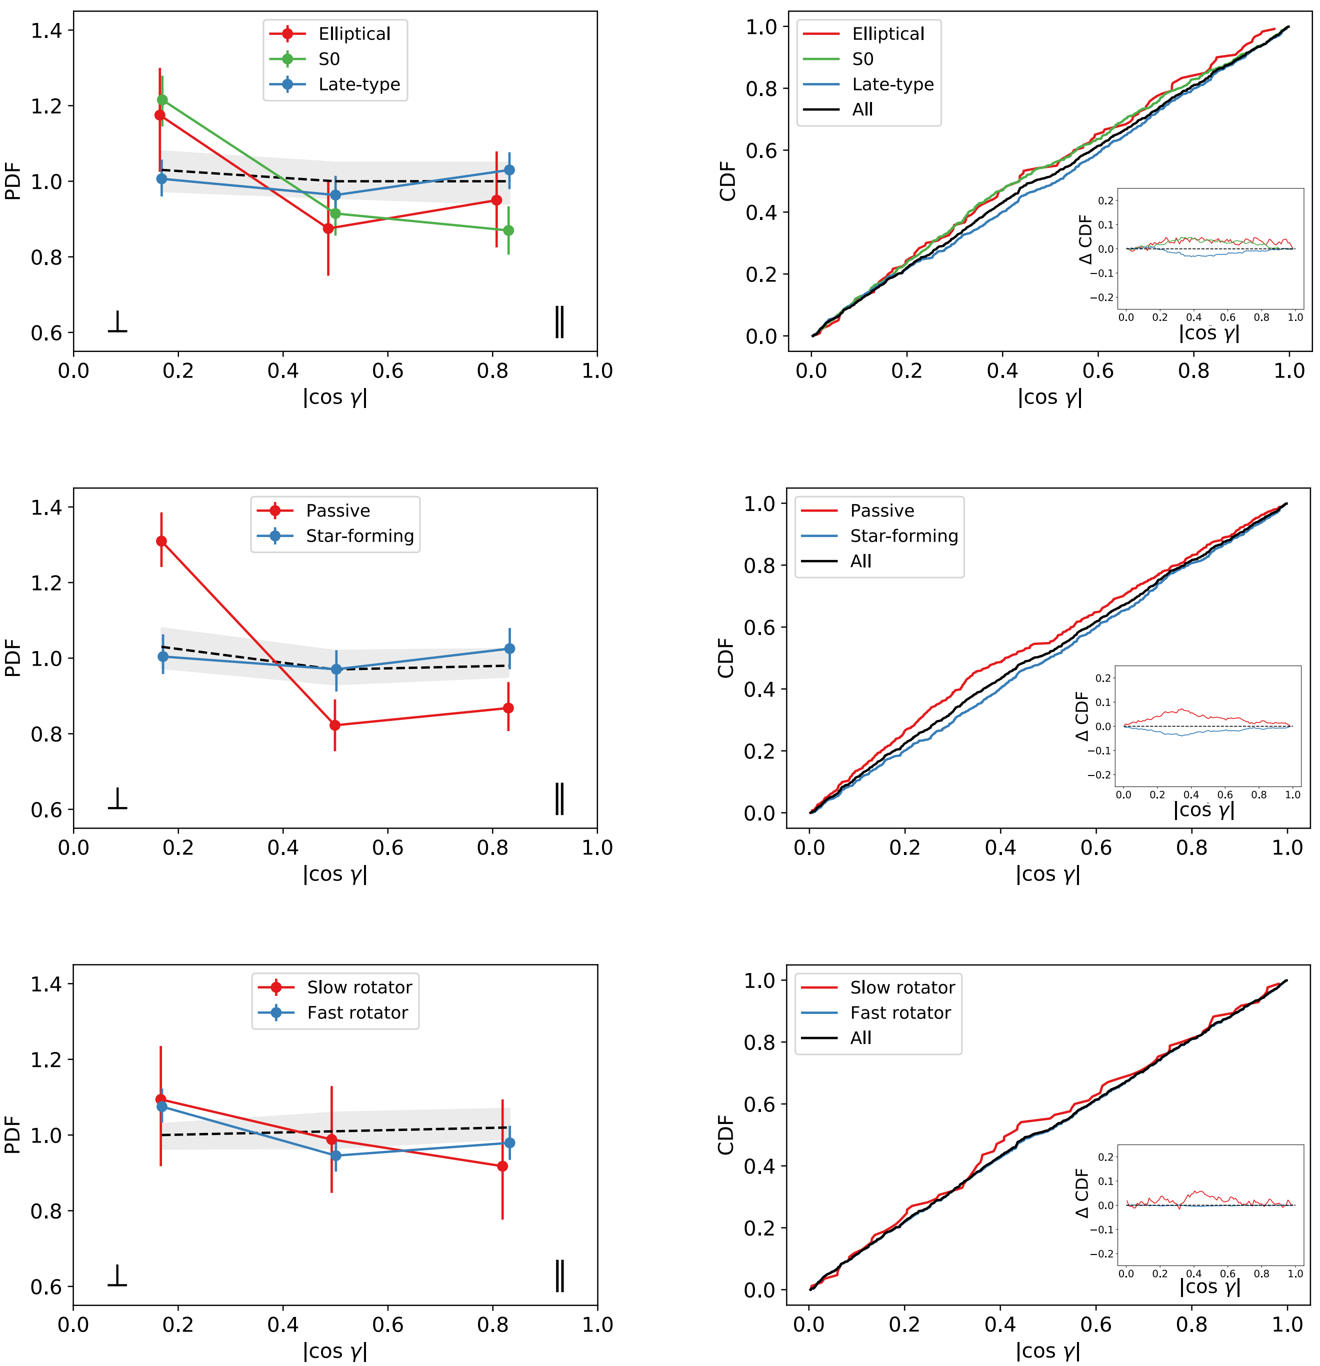


**Figure S5:** PDFs (left) and CDFs (right) of the spin–filament alignments for the SAMI galaxies divided according to visual morphology (top), spectral classification (middle) and kinematic morphology (bottom). A statistically significant perpendicular alignment is found for S0 galaxies and passive galaxies; hints of a similar tendency are seen for the smaller sample of ellipticals and slow rotators. Late-type galaxies, star-forming galaxies, and fast rotators are consistent with uniform PDFs. A significant difference is detected between the $|\cos\gamma|$ distributions of ellipticals+S0s and late-types, and also between passive and star-forming galaxies.
